# Supplementary material for: Elderly HealthMag: Systematic Building and Calibrating a Tool for Identifying and Evaluating Senior User Digital Health Software
Source: arXiv:2601.22627 source file (2026-01-30)
Supplement: Supplementary file 1 [file 20_Personas.pdf]

### Persona 1 (Male, 65–70 years old, Theme 1, preferred language: Mandarin)

- **Demographic Information:** Name: Zhao, 68 years old, male.
- **Current Situation:** Retired, enjoys travelling, and often joins senior travel groups.
- **Personal Background:** Former corporate employee with a high school education. Lives with his wife; his children work in other cities and keep in touch via phone.
- **Health and Wellness:** Has hypertension, requires regular blood pressure monitoring, and takes medication. Exercises by walking.
- **Information-Seeking Behaviour:** Searches online for hypertension-related health knowledge but is uncertain about its accuracy. Trusts doctors' advice more.
- **Attitude Toward Technology:** Uses a smartphone for calls and photos. Interested in e-health apps but worried about complex operations.
- **Pain Points and Motivations:**
  - **Pain Point:** Concerned about forgetting medication and affecting his health.
  - **Motivation:** Hopes to use a smartphone app to better manage health by recording blood pressure data and setting medication reminders.
- **Scenario:** Zhao plans to travel with his wife but is worried about forgetting his hypertension medication. He downloads a health app but encounters difficulties setting up medication reminders. He tries to follow the instructions, hoping to resolve it before the trip for stable blood pressure management.

### Persona 2 (Female, 65–70, Theme 2, preferred language: English)

- **Demographic Information:** Name: Joyce, 66, female.
- **Current Situation:** Retired, loves gardening, and often shares tips with neighbours.
- **Personal Background:** Homemaker, raised children who now live nearby and visit often.
- **Health and Wellness:** Generally healthy but occasionally experiences joint pain and tries simple remedies.
- **Information-Seeking Behaviour:** Reads health articles on her phone, discusses remedies with neighbours, and consults community doctors.
- **Attitude Toward Technology:** Comfortable using smartphones and interested in apps that offer health and exercise advice.
- **Pain Points and Motivations:**
  - **Pain Point:** Joint pain disrupts daily activities.
  - **Motivation:** Wants an app to find effective joint care methods, reduce pain, and better care for her plants.
- **Scenario:** While gardening, Joyce's joint pain worsens. She recalls seeing a health app with joint care content and tries to find exercises suited to her. She struggles to sift through the vast content but hopes to quickly find effective advice to alleviate her pain.

### Persona 3 (Male, 71–75, Theme 4, preferred language: English)

- **Demographic Information:** Name: Frank, 73, male.

- **Current Situation:** Retired teacher, enjoys reading and occasionally attends reunions.
- **Personal Background:** Holds a bachelor's degree, taught for many years, lives alone since his spouse passed away, and relies on his children for care.
- **Health and Wellness:** Has mild diabetes and declining eyesight, requiring dietary control and regular blood sugar checks.
- **Information-Seeking Behavior:** Prefers printed materials and consultations with doctors over smartphone-based health information.
- **Attitude Toward Technology:** Uses a smartphone for news but is unfamiliar with health app functionalities, fearing errors.
- **Pain Points and Motivations:**
  - **Pain Point:** Poor eyesight makes smartphone use difficult.
  - **Motivation:** Seeks a user-friendly app to log blood sugar levels and provide dietary advice tailored to his vision limitations.
- **Scenario:** After a hospital checkup, Frank's doctor recommends better blood sugar tracking. He remembers his children suggesting an app for this but struggles with input due to his eyesight, becoming anxious while trying to find a solution for accurate tracking.

#### **Persona 4 (Female, 71–75, Theme 4, preferred language: English)**

- **Demographic Information:** Name: Mary, 72, female.
- **Current Situation:** Retired factory worker, active in square dancing groups.
- **Personal Background:** Worked in a factory for many years, has a middle school education, lives with her husband, and enjoys visits from her children.
- **Health and Wellness:** Generally healthy but cautious about injuries during dancing, does simple warm-up exercises.
- **Information-Seeking Behavior:** Exchanges fitness tips with her dance group and watches fitness videos online.
- **Attitude Toward Technology:** Uses smartphones for videos and messaging, seeks apps with safety tips and dance tutorials.
- **Pain Points and Motivations:**
  - **Pain Point:** Fear of injuries affecting her participation in dancing.
  - **Motivation:** Desires an app with reliable warm-up and injury prevention techniques to enjoy dancing safely.
- **Scenario:** Preparing for a dance competition, Mary worries about increased training intensity and injuries. She downloads several apps for guidance but struggles to find trustworthy information. She is determined to identify reliable advice for effective warm-ups.

#### **Persona 5 (Male, 71 - 75 years old, Theme 4, preferred language: Italian)**

**Demographic Information:** Name: Marco, 73 years old, Male.

**Current Situation:** After retirement, he enjoys fishing and often goes alone to fishing spots by the river.

**Personal Background:** He was a self-employed businessman with a stable financial background. His children work locally, and family relationships are

harmonious.

**Health and Wellness:** Generally healthy, but he feels back and waist pain after sitting for long periods while fishing.

**Information-Seeking Behaviour:** Occasionally exchanges tips on relieving discomfort with fellow anglers but is not proactive in searching for information online.

**Attitude Toward Technology:** He can use a smartphone for navigation to fishing spots, but is not interested in other features and feels that monitoring apps might invade his privacy.

**Pain Points and Motivations:**

**Pain Point:** Discomfort from sitting too long while fishing affects his subsequent activities.

**Motivation:** He would like simple life-monitoring devices or apps that remind him to move occasionally, prevent health issues from prolonged sitting, and not interfere with the enjoyment of fishing.

**Scenario:** Marco goes fishing by the river again, sitting for several hours. After returning home, his back and waist pain are worse than before. He recalls that a fellow angler mentioned devices that can monitor sitting time and remind him to move. He hesitates to explore it, worried it might be complicated or invade his privacy, but he does want to improve the situation so that he can continue enjoying fishing.

---

**Persona 6 (Female, 65 - 70 years old, Theme 2, preferred language: greek)**

**Demographic Information:** Name: Katerina, 65 years old, Female.

**Current Situation:** Retired and staying at home, enjoys doing handicrafts, and frequently participates in community craft activities.

**Personal Background:** A housewife skilled in handicrafts, her children are very filial and often accompany her.

**Health and Wellness:** Occasionally suffers from insomnia and has tried various folk remedies for sleep.

**Information-Seeking Behaviour:** She exchanges experiences and solutions for insomnia with other elderly people in the community and watches health programs on television for information.

**Attitude Toward Technology:** She has a basic understanding of smartphones and is curious about sleep-monitoring apps, but is unsure if they are reliable.

**Pain Points and Motivations:**

**Pain Point:** Insomnia affects her mental state and handicraft productivity.

**Motivation:** She wants to use sleep-monitoring apps to understand her sleep issues, find effective solutions, improve her sleep quality, and be more focused on her craft creations.

**Scenario:** Katerina's insomnia has worsened recently, and she frequently makes mistakes while doing crafts. She sees a community advertisement about devices and apps that monitor sleep and decides to give them a try. With her children's help, she

downloads the app and prepares to use it. However, she feels uncomfortable wearing the monitoring device and is unsure if she should continue. She hopes to find a suitable way to wear it and understand her sleep situation better.

---

**Persona 7 (Male, 71 - 75 years old, Theme 2, preferred language: English)**

**Demographic Information:** Name: Ahmed, 74 years old, Male.

**Current Situation:** A retired official who enjoys calligraphy and painting, often creating in his study.

**Personal Background:** Highly cultured, his children work out of town, and his wife is in poor health and requires his care.

**Health and Wellness:** Suffers from mild arthritis that affects hand movements and requires rehabilitation exercises.

**Information-Seeking Behaviour:** Consults doctors for advice on arthritis rehabilitation and reads medical books.

**Attitude Toward Technology:** Interested in some health-monitoring features of smartphones but feels the operations are complicated and wishes for something simpler.

**Pain Points and Motivations:**

Pain Point: Arthritis limits hand movements, affecting his calligraphy and painting.

Motivation: He hopes for life-monitoring and rehabilitation guidance apps to help with recovery exercises, reduce arthritis symptoms, restore hand flexibility, and continue creating calligraphy and paintings.

**Scenario:** Ahmed is working on a calligraphy piece when the pain from arthritis in his hands becomes unbearable, forcing him to stop. He recalls that a doctor mentioned using technology to assist in rehabilitation. He tries searching for related apps on his smartphone and, after downloading them, struggles to understand many of the functions. He works hard to learn how to use them, hoping to find a suitable rehabilitation program to alleviate hand pain and complete his work.

---

**Persona 8 (Female, 65 - 70 years old, Theme 4, preferred language: English)**

**Demographic Information:** Name: Margaret, 68 years old, Female.

**Current Situation:** A retired nurse who enjoys walking and participating in community volunteer activities is concerned about the health status of elderly people in her community.

**Personal Background:** A professional nurse, her children work locally, her husband has passed away, and she lives independently.

**Health and Wellness:** Her health is generally good, but she worries that as she ages, any sudden health problems might go unnoticed.

**Information-Seeking Behaviour:** She follows medical journals and community health lectures, and is sensitive to new health-monitoring technologies.

**Attitude Toward Technology:** Skilled in using smartphones and values apps that

can provide emergency monitoring and notifications.

**Pain Points and Motivations:**

**Pain Point:** Fears that she may not receive timely assistance in case of a sudden health issue.

**Motivation:** She wants a reliable life-monitoring system that can notify community staff or her children in case of a health problem, ensuring her safety and allowing her to participate in community activities with peace of mind.

**Scenario:** While attending a community volunteer event, Margaret hears about an elderly person who suffered from a sudden illness at home, and the lack of timely help delayed treatment. She relates this to her own situation and decides to find a suitable life-monitoring app. She browses through the app store, comparing the features and reviews of different apps, hoping to find one that can accurately monitor her health and notify people quickly, ensuring her safety and the safety of other elderly individuals in the community.

**Persona 9 (Male, 76-80 years old, Theme 3, preferred language: Vietnamese)**

**Demographic Information:** Name: Minh, 78 years old, male.

**Current Situation:** His health is average, with hearing loss. He enjoys listening to the radio. His children live far away, and he relies on his spouse for companionship.

**Personal Background:** He was a regular worker, with low education. He has a deep relationship with his spouse and has lived in the local area all his life.

**Health and Wellness:** In addition to hearing problems, he also has some chronic diseases that require regular medication.

**Information-Seeking Behavior:** He mainly obtains information through television and radio and is not familiar with new social technologies.

**Attitude Toward Technology:** He is not very skilled in using smartphones and has some anxiety about social apps, feeling that he won't be able to learn them.

**Pain Points and Motivations:**

- **Pain Point:** Hearing loss makes communication difficult, leading to feelings of loneliness.
- **Motivation:** He hopes for a simple social app or device that makes it easier to communicate with his children and friends, alleviating loneliness and allowing better communication despite his hearing loss.

**Scenario:** Minh's children bought him a smartphone to make video calls easier. However, he feels lost when faced with the phone and doesn't know how to answer a video call. He is eager to talk to his children but worries about not being able to learn, which might disappoint them. He tries to follow his children's instructions, hoping to successfully answer a video call and have a good conversation with them.

---

Persona 10 (Female, 76-80 years old, Theme 3, preferred language: English)

**Demographic Information:** Name: Diane, 77 years old, female.

**Current Situation:** Her spouse has passed away, and her children are busy with work. She lives alone and enjoys reminiscing about the past.

**Personal Background:** A housewife, she has worked hard all her life. She has several good friends nearby, but they don't meet often.

**Health and Wellness:** She is physically weak and has difficulty moving, requiring care.

**Information-Seeking Behaviour:** She chats with visiting friends about her past life and doesn't actively seek out new information.

**Attitude Toward Technology:** She knows a little about smartphones and can make and receive calls, but is not familiar with social apps and is eager to learn.

**Pain Points and Motivations:**

- **Pain Point:** She feels very lonely and lacks companionship.
- **Motivation:** She hopes to use social apps to communicate more with her children and friends, share memories, and reduce her loneliness, while receiving more emotional care.

**Scenario:** Diane saw her neighbour video chatting with her child who lives far away, and was envious. She asked her neighbour to teach her how to use the video chat app. During the learning process, she kept forgetting the steps, feeling anxious. She hopes to learn quickly so she can often video chat with her children to ease her longing for them.

---

Persona 11 (Male, 81-85 years old, Theme 3, Preferred Language: Italian)

**Demographic Information:** Name: Giovanni, 83 years old, male.

**Current Situation:** He is physically weak and spends most of his time lying in bed. His children take turns caring for him, and he has little social activity.

**Personal Background:** He was a farmer and lived a simple life. He has a good relationship with his children, but due to his health, he has little contact with the outside world.

**Health and Wellness:** He suffers from multiple illnesses and requires long-term care.

**Information-Seeking Behaviour:** He doesn't actively seek information and relies on his children to inform him about external matters.

**Attitude Toward Technology:** He is completely unfamiliar with smartphones and modern technology and doesn't have the energy to learn.

**Pain Points and Motivations:**

- **Pain Point:** He is extremely lonely due to being bedridden and longs to communicate with others.
- **Motivation:** He hopes for a simple way to communicate with his family and friends, even if it's just a simple greeting, to feel warmth and care and alleviate his loneliness.

**Scenario:** Giovanni's grandson visited him and showed him some family photos and videos. Giovanni was happy and wished he could see them more often. His grandson

wanted to teach him how to use a tablet to view the photos, but Giovanni felt he wouldn't be able to learn and didn't want to disappoint his grandson. With his grandson's patient guidance, Giovanni tried to operate the tablet, hoping to see more family images to comfort his heart.

---

### **Persona 12 (Female, 81-85 years old, Theme 3, Preferred Language: Greek)**

**Demographic Information:** Name: Sophia, 82 years old, female.

**Current Situation:** She lives in a nursing home, and her children visit her regularly. She gets along well with some of the other elderly residents.

**Personal Background:** A housewife, her children placed her in the nursing home due to their busy work schedules, and she understands their difficulties.

**Health and Wellness:** She has some age-related illnesses and needs care from nursing staff.

**Information-Seeking Behaviour:** She attends health lectures in the nursing home to gain knowledge about health and social topics.

**Attitude Toward Technology:** She has some impression of smartphones and is curious when she sees others using them, but doesn't know how to operate them.

**Pain Points and Motivations:**

- **Pain Point:** At times, she misses her family and hopes to stay in touch.
- **Motivation:** She hopes to learn how to use simple social apps to communicate easily with her children and friends, and better integrate into the social life of the nursing home, reducing her feelings of longing.

**Scenario:** Sophia saw other elderly residents in the nursing home using their phones to video chat with their families, and she really wanted to do the same. She asked the staff for help, hoping they could teach her how to use the video chat function. During the learning process, she encountered many difficulties, such as not being able to see the screen clearly and pressing the wrong buttons. However, she persisted in learning, hoping to be able to video call her family soon.

### **Persona 13 (male, 65-70, Theme 5, Preferred Language: English)**

**Demographic Information:**

Name: Brian, 66 years old, Male.

**Current Situation:**

Retired at home, enjoys playing chess, and often plays with old friends in the community's chess room. His children work in other cities, and his wife is not in good health and needs his care.

**Personal Background:**

He was a factory worker and had considerable life experience. He has good relationships with the neighbours in his community, and the community staff is familiar with his family situation.

**Health and Wellness:**

He is generally in good health but occasionally experiences dizziness, possibly due to blood pressure fluctuations.

**Information-Seeking Behavior:**

He regularly goes to the community hospital to have his blood pressure checked, follows the doctor's advice to adjust his lifestyle, and also shares wellness tips with his chess friends.

**Attitude Toward Technology:**

He knows how to use a smartphone to make calls and send messages. He is interested in health-monitoring apps but doesn't know how to operate them well.

**Pain Points and Motivations:**

**Pain Point:** He worries that if he suddenly feels unwell, his wife won't be able to get help in time.

**Motivation:** He hopes for an emergency call device or app that can quickly connect him with community workers or his children when he experiences dizziness or other sudden issues. He also wants a system that will notify others if his wife needs assistance, ensuring the safety and happiness of his family.

**Scenario:**

While playing chess, Brian suddenly felt dizzy. He wanted to use his phone to contact his children, but found it difficult to operate due to his dizziness. He remembered that the community had promoted an emergency call button, but he hadn't yet installed it. He tried to calm himself down and asked his chess friend for help, hoping they could contact his family or community staff. He also decided to install the emergency call device as soon as he got home to prevent a similar situation in the future.

**Persona 14 (Female, 65–70 years old, Theme 5, Preferred Language; English)**

- **Demographic Information:**  
Name: Lin, 68 years old, Female.
- **Current Situation:**  
Retired teacher, enjoys walking and reading, lives alone in an apartment, and her children visit her once or twice a week.
- **Personal Background:**  
Has a high level of education, worked in the education field for many years, has many former students, and maintains contact with them. She is also respected in the community.
- **Health and Wellness:**  
Her vision has deteriorated, and sometimes she stumbles while walking because she can't see the path clearly. She also has mild osteoporosis.
- **Information-Seeking Behavior:**  
She reads books on health and wellness and attends community health seminars to learn about fall prevention and other related topics.
- **Attitude Toward Technology:**  
She is quite proficient with smartphones, uses them to read e-books and check the

news. She is interested in smart wearable devices that can provide fall alerts, but she is concerned about the high cost.

- **Pain Points and Motivations:**

Pain Point: She is afraid of falling and injuring herself while walking, but doesn't want to reduce her physical activity.

Motivation: She hopes to have a fall alert device or app that can warn her of fall risks and notify her family or community workers, allowing her to continue walking and exercising with peace of mind while maintaining a healthy lifestyle.

- **Scenario:**

Lin was walking in the evening when, due to the low light, she almost tripped over a stone by the roadside. She was shaken by the experience and remembered seeing an introduction to fall alert devices. After returning home, she searched online for relevant products and found that the prices varied widely. She contacted her children, hoping they could help her choose a cost-effective option, so she could feel safer during her next walk and not worry about falling and getting injured.

### **Persona 15 (Male, 71–75 years old, Theme 4, Preferred Language: Mandarin)**

- **Demographic Information:** Name: David, 73 years old, Male.
- **Current Situation:** Enjoys studying history and culture in retirement, often visiting libraries and conducting online research.
- **Personal Background:** Former cultural worker with a university education, passionate about knowledge. His children, also in cultural fields, often discuss academic topics with him.
- **Health and Wellness:** Generally healthy but experiences eye strain from prolonged reading or screen use.
- **Information-Seeking Behaviour:** Frequently searches for materials on academic websites and cultural forums, valuing accuracy and authority.
- **Attitude Toward Technology:** Familiar with computers and smartphones but less knowledgeable about advanced search and knowledge management technologies.
- **Pain Points and Motivations:**
  - Pain Points:* Struggles to quickly and accurately find relevant historical and cultural resources amid vast amounts of information.
  - Motivations:* Seeks intelligent search and knowledge management systems to filter information precisely according to his needs, present it in an easy-to-read format, reduce eye strain, and improve research efficiency.
- **Scenario:** While writing an article on ancient culture, David struggled with the overwhelming amount of irrelevant search results online. Intrigued by intelligent search tools that promise greater accuracy, he explored their use, hoping to find reliable resources efficiently and complete his article smoothly.

### **Persona 16 (Female, 71–75 years old, Theme 5, Preferred Language: English)**

- **Demographic Information:**

Name: Joanna, 72 years old, Female.
- **Current Situation:**

Retired and living at home, enjoys gardening and participating in community craft activities, lives with her spouse, and her children are all married and live nearby.

- **Personal Background:**  
A housewife, skilled in crafts and gardening, often shares her gardening experiences and handmade crafts with other elderly people in the community, and has close relationships with her neighbors.
- **Health and Wellness:**  
Her health is average, suffers from arthritis, and experiences joint pain after prolonged activity, making movement difficult, especially when going up and down stairs.
- **Information-Seeking Behavior:**  
She consults doctors about treatments for arthritis, tries folk remedies, and exchanges rehabilitation experiences with other elderly people suffering from arthritis in the community.
- **Attitude Toward Technology:**  
She can use a smartphone to make calls and check information. She is interested in smart devices that can contact family members and community services in emergencies, but is concerned about the complexity of operation and fears she won't be able to learn it.
- **Pain Points and Motivations:**  
Pain Point: She is concerned about falling while going up or down stairs, or when home alone, due to arthritis flare-ups, and being unable to get help quickly.  
Motivation: She hopes to have a simple and easy-to-use emergency contact device or app that can quickly notify family members or community workers if she experiences joint pain or falls, allowing her to live safely at home and participate in community activities.
- **Scenario:**  
Joanna was moving a flowerpot from the balcony to the living room when, due to joint pain, she nearly slipped and fell. She grabbed a nearby table to steady herself, and after a moment, realised that a fall could be very dangerous, and she would have difficulty contacting her family in time. She decided to have her children help her find a simple emergency call button to be installed in a visible and easily accessible location, so that she can quickly ask for help in similar situations and ensure her safety.

#### **Persona 17 (Male, 76–80 years old, Theme 1, preferred language: English)**

- **Demographic Information:** Name: Ben, 78 years old, Male.
- **Current Situation:** Suffers from heart disease and diabetes, requiring regular hospital visits and medication, spending most time resting at home.
- **Personal Background:** Former factory worker with a regular lifestyle. His devoted children take turns caring for him.
- **Health and Wellness:** Weak health necessitates a strict diet, medication adherence, monitoring of blood sugar and blood pressure, and being allergic to penicillin.
- **Information-Seeking Behaviour:** Relies on doctors for advice and occasionally reads health-related books.

- **Attitude Toward Technology:** Unfamiliar with smartphones and skeptical of medical apps, preferring hospital equipment and expert opinions.
- **Pain Points and Motivations:**

*Pain Points:* Inconvenience of hospital visits and concern over emergencies at home.

*Motivations:* Desires a medical assistance system for hospital appointment bookings, medication reminders, health monitoring, and emergency alerts to notify family or doctors for better health management.
- **Scenario:** With his children busy at work, Mr. Zhu found hospital visits challenging. He heard about online appointment systems and asked his children to help install the app. Despite finding it complex, he persisted in learning, aiming to manage appointments independently and stay on top of his healthcare.

**Persona 18 (Female, 76–80 years old, Theme 2, preferred language: Punjabi)**

- **Demographic Information:** Name: Kamala, 77 years old, Female.
- **Current Situation:** Struggles with osteoporosis, and second type of diabetes, and cataracts, requires a cane, and attends regular rehabilitation therapy sessions.
- **Personal Background:** Homemaker with children nearby who became more attentive after her spouse's passing.
- **Health and Wellness:** Fragile bones necessitate safety precautions, calcium supplementation, and guided exercises.
- **Information-Seeking Behavior:** Consults doctors about rehabilitation and diet, exchanging advice with peers facing similar issues.
- **Attitude Toward Technology:** Knows basic smartphone functions and is interested in rehabilitation and health monitoring apps but doubts their professional reliability.
- **Pain Points and Motivations:**

*Pain Points:* Concern over improper exercise techniques worsening her condition.

*Motivations:* Looks for a professional rehabilitation app offering personalized exercise plans and monitoring to ensure safety and effectiveness.
- **Scenario:** During rehabilitation, Kamala worried her methods might be incorrect. Recalling a health app with rehabilitation guidance, she asked her children for help accessing it. Unsure which videos suited her condition, she sought support from the app's customer service or a specialist for accurate advice.

**Persona 19 (Male, 81–85 years old, Theme 2, preferred language: Germany)**

- **Demographic Information:** Name: Karl, 83 years old, Male.
- **Current Situation:** Bedridden with chronic illnesses such as hypertension and hyperlipidemia, requiring constant care.
- **Personal Background:** Former soldier with a rich life history, cared for devotedly by his children.
- **Health and Wellness:** Long-term immobility increases the risk of complications like bedsores, requiring meticulous care and health monitoring.
- **Information-Seeking Behavior:** Relies entirely on family and healthcare providers for information.
- **Attitude Toward Technology:** Unfamiliar with technology and unable to use it independently.

- **Pain Points and Motivations:**

*Pain Points:* Concerns over inadequate care leading to complications and an inability to communicate needs.

*Motivations:* Wishes for an intelligent monitoring system to track health metrics, remind caregivers of necessary actions like repositioning, and alert doctors during emergencies to ensure safety.

- **Scenario:** Despite diligent care, occasional oversights occurred. Hearing about smart monitoring devices, his family decided to try one. While setting it up, they worried about its precision and comfort. They adjusted the system carefully to improve care quality and minimize risks.

**Persona 20 (Female, 86+ years old, Theme 2, preferred language: Cantonese)**

- **Demographic Information:** Name: Wai-Ling, 88 years old, Female.
- **Current Situation:** Extremely frail, residing in a nursing home with 24-hour care in a semi-comatose state.
- **Personal Background:** Homemaker who raised children now elderly themselves and less frequent visitors.
- **Health and Wellness:** Multiple organ failures sustained through medication and nutrition.
- **Information-Seeking Behavior:** Incapable of seeking information actively.
- **Attitude Toward Technology:** Unable to use any technological devices.
- **Pain Points and Motivations:**

*Pain Points:* Needs advanced monitoring and care to detect and respond to changes promptly.

*Motivations:* Hopes for sophisticated nursing systems in the facility to monitor vital signs, swiftly detect changes, and ensure comfort in her final days.
- **Scenario:** The nursing staff closely monitored her condition, but traditional methods sometimes lagged. They considered adopting advanced monitoring systems. While concerned about accuracy, they carefully implemented the system to provide her with better care and reduce discomfort in her final moments.
