# Supplementary material for: Elderly HealthMag: Systematic Building and Calibrating a Tool for Identifying and Evaluating Senior User Digital Health Software
Source: arXiv:2601.22627 source file (2026-01-30)
Supplement: Supplementary file 2 [file Interview_guide.pdf]

# Interview guide for ERM project 47930

This is the interview guide for project 47930. In this guide, we will state the research questions that we plan to answer and the process guide for the interview step by step.

1. **Research Questions:** What and how facets of health conditions of users influence their use of digital health Apps?
  - Sub-RQ1: Will users' health conditions influence experience in using digital health Apps due to interviewees' experience?
  - Sub-RQ2: What are the facets that affect the digital health experience of users due to interviewees' experience?
  - Sub-RQ3: Do the proposed facets and personas make a good representation of such inclusiveness of health conditions?
2. **Process:**
  - Step 1: Ask the interviewee to introduce themselves about their experience in digital health software. Based on their experience, either explain what InclusiveMag is first(if no HCI experience at all), or just introduce HealthMag(if with HCI experience). HealthMag is a derivative of InclusiveMag<sup>[1]</sup>.
  - Step 2: Ask Questions 1-3, and then show potential facets, and then ask Questions 4-5.
  - Step 3: Show some examples of potential InclusiveMag Personas designed by us and ask Questions 6-8.
3. **Interview Questions:**

| Question Index | Question                                                                                                                                                                                                        | Time (/mins) | Related sub-RQ(s) |
|----------------|-----------------------------------------------------------------------------------------------------------------------------------------------------------------------------------------------------------------|--------------|-------------------|
| 1              | (depends on their research focus/experience) Have you ever seen any challenges that influence users' health outcomes or their user experience because of their health conditions, according to your experience? | 5            | 1                 |
| 2              | Would you say Health Conditions have impact on UX in digital health Apps? And why do you think that?                                                                                                            | 5            | 1                 |
| 3              | What will influence digital health Apps' user experience in your opinion, other than users' health conditions? (Do you think they have a correlated influence?)                                                 | 5            | 1,2               |
| 4              | (After showing the potential facets of health and Age to the interviewee), Could you rank these 7 facets based on how important they are? Why do you rank it like that?                                         | 10           | 2                 |
| 5              | Are there any facets here that you think are not relevant or redundant with others? Are there any important factors we're missing that should be considered as separate facets?                                 | 5            | 2                 |
| 6              | (After showing the potential personas to the interviewee), Do you think those personas look good/real to you based on your experience?                                                                          | 3            | 3                 |
| 7              | Do you think those personas can represent different health conditions of users to you? How would you improve them?                                                                                              | 7            | 3                 |
| 8              | Is there anything else you would like to comment on this topic?                                                                                                                                                 | 5            | 1,2,3             |
| In total       |                                                                                                                                                                                                                 | 45           |                   |

## 4. Potential facets and personas:

- **Facets for Health dimension**

|                                                |
|------------------------------------------------|
| Health Motivation for using Digital health App |
|------------------------------------------------|

|                            |
|----------------------------|
| Cognitive (dys)function    |
| Caregiver Support received |
| Physical difficulties      |
| Medical self-efficacy      |
| Trust towards Technology   |
| Technical Proficiency      |

- **Facets for Older Adults(Age) dimension**

|                                                                                               |
|-----------------------------------------------------------------------------------------------|
| Technical Proficiency                                                                         |
| Emotions                                                                                      |
| Visual impairment                                                                             |
| Social Influence on Technology: eg. their caregivers uses Tech, their family/friends use Tech |
| Physical difficulties                                                                         |

- **Examples of potential InclusiveMag Personas: [2]-[4]**

#### **References:**

[1] C. Mendez, L. Letaw, M. Burnett, S. Stumpf, A. Sarma and C. Hilderbrand, "From GenderMag to InclusiveMag: An Inclusive Design Meta-Method," 2019 IEEE Symposium on Visual Languages and Human-Centric Computing (VL/HCC), Memphis, TN, USA, 2019, pp. 97-106, doi: 10.1109/VLHCC.2019.8818889. keywords: {Software;Sociology;Statistics;Systematics;Information processing;Visualization;Diversity;InclusiveMag},
